# Supplementary material for: Golden Noise for Diffusion Models: A Learning Framework
Source: arXiv:2411.09502 source file (2025-07-17)
Supplement: Supplementary file 1 [file clip_mps.tex]

% Please add the following required packages to your document preamble:
% \usepackage{multirow}
% \usepackage[table,xcdraw]{xcolor}
% Beamer presentation requires \usepackage{colortbl} instead of \usepackage[table,xcdraw]{xcolor}
\begin{table*}[!ht]
\begin{center}

\caption{Quantitative comparison of NPNet on SDXL over various datasets.}

\setlength{\tabcolsep}{10pt}
\resizebox{1.0\linewidth}{!}{%
\begin{tabular}{c|c|ccc|ccc|ccc}
\hline
 &  & \multicolumn{3}{c|}{Pick-a-Pic} & \multicolumn{3}{c|}{DrawBench} & \multicolumn{3}{c}{HPD v2} \\ \cline{3-11} 
\multirow{-2}{*}{Model} & \multirow{-2}{*}{Metric} & Standard & Inversion & NPNet~(ours) & Standard & Inversion & NPNet~(ours) & Standard & Inversion & NPNet~(ours) \\ \hline
 & CLIPScore & 82.04 & 82.5 & \CC84.08 & 80.77 & 80.81 & \CC81.53 & 87.34 & 87.08 & \CC88.12 \\
\multirow{-2}{*}{SDXL} & MPS & - & 51.41 & \CC52.14 & - & 51.98 & \CC53.70 & - & 53.03 & \CC56.02 \\ \hline
 & CLIPScore & 82.67 & 82.77 & \CC89.58 & 81.86 & 81.89 & \CC82.24 & 88.68 & 89.12 & \CC89.42 \\
\multirow{-2}{*}{DreamShaper-xl-v2-turbo} & MPS & - & 49.14 & \CC52.34 & - & 46.62 & \CC53.53 & - & 46.94 & \CC52.49 \\ \hline
 & CLIPScore & 80.37 & 80.21 & \CC81.01 & 79.40 & 79.55 & \CC80.75 & 85.68 & 86.17 & \CC86.94 \\
\multirow{-2}{*}{Hunyuan-DiT} & MPS & - & 49.08 & \CC51.60 & - & 49.25 & \CC51.93 & - & 51.63 & \CC52.87\\
\bottomrule
\end{tabular}
}
\label{table:clip_mps}
\end{center}
\end{table*}
